# Supplementary material for: explAIner: A Visual Analytics Framework for Interactive and Explainable Machine Learning
Source: arXiv:1908.00087 source file (2019-10-07)
Supplement: Supplementary file 1 [file supplementary.tex]

\section*{Supplementary Related Work}
\begin{table*}[ht!]
\centering
\begin{tabular}{|l|l|l|l|l|l|l|l|l|}
\hline
\multicolumn{1}{|c|}{\multirow{2}{*}{VA Approach}} & \multicolumn{1}{c|}{\multirow{2}{*}{Reference}} & \multicolumn{4}{c|}{Task}                          & \multicolumn{3}{c|}{Operation Level} \\ \cline{3-9} 
\multicolumn{1}{|c|}{}                             & \multicolumn{1}{c|}{}                           & Underst. & Diagnosis & Refinement & Reporting & Data     & Surrogate     & Model     \\ \hline
Node-Link Vis              & Harley~\cite{Harley2015imageinterpreter} & \tikzcircle{2pt}                                 & \tikzcircle[black, fill=white]{2pt}                             & \tikzcircle[black, fill=white]{2pt}                        & \tikzcircle[black, fill=white]{2pt}                             & \tikzcircle{2pt}/\tikzcircle[black, fill=white]{2pt}                        & \tikzcircle[black, fill=white]{2pt}                                   & \tikzcircle{2pt}                         \\ \hline
Prospector                 & Krause et al.~\cite{Krause2016} & \tikzcircle{2pt}                                 & \tikzcircle{2pt}                             & \tikzcircle[black, fill=white]{2pt}                        & \tikzcircle[black, fill=white]{2pt}                             & \tikzcircle{2pt}                        & \tikzcircle[black, fill=white]{2pt}                                   & \tikzcircle{2pt}                         \\ \hline
CNNVis                     & Liu et al.~\cite{Liu2016} & \tikzcircle{2pt}                                 & \tikzcircle{2pt}                             & \tikzcircle{2pt}                        & \tikzcircle[black, fill=white]{2pt}                             & \tikzcircle{2pt}                        & \tikzcircle[black, fill=white]{2pt}                                   & \tikzcircle{2pt}                         \\ \hline
Hidden Activity Vis        & Rauber et al.~\cite{Rauber16} & \tikzcircle{2pt}                                 & \tikzcircle{2pt}                             & \tikzcircle[black, fill=white]{2pt}                        & \tikzcircle[black, fill=white]{2pt}                             & \tikzcircle{2pt}                        & \tikzcircle[black, fill=white]{2pt}                                   & \tikzcircle{2pt}                         \\ \hline
TensorFlow Playground        & Smilkov et al.~\cite{Smilkov2016tensorflowplayground} & \tikzcircle{2pt}                                 & \tikzcircle{2pt}                             & \tikzcircle{2pt}                        & \tikzcircle[black, fill=white]{2pt}                             & \tikzcircle{2pt}                        & \tikzcircle[black, fill=white]{2pt}                                   & \tikzcircle{2pt}                         \\ \hline
DeepEyes                   & Pezzoti et al.~\cite{Pezzotti2017} & \tikzcircle{2pt}                                 & \tikzcircle{2pt}                             & \tikzcircle{2pt}                        & \tikzcircle[black, fill=white]{2pt}                             & \tikzcircle{2pt}                        & \tikzcircle[black, fill=white]{2pt}                                   & \tikzcircle{2pt}                         \\ \hline
RNNVis                     & Ming et al.~\cite{Ming2018} & \tikzcircle{2pt}                                 & \tikzcircle{2pt}                             & \tikzcircle[black, fill=white]{2pt}                        & \tikzcircle[black, fill=white]{2pt}                             & \tikzcircle{2pt}                        & \tikzcircle[black, fill=white]{2pt}                                   & \tikzcircle{2pt}                         \\ \hline
DGMTracker                 & Liu et al.~\cite{Liu2018} & \tikzcircle{2pt}                                 & \tikzcircle{2pt}                             & \tikzcircle[black, fill=white]{2pt}                        & \tikzcircle[black, fill=white]{2pt}                             & \tikzcircle{2pt}                        & \tikzcircle[black, fill=white]{2pt}                                   & \tikzcircle{2pt}                         \\ \hline
Class Hierarchy?           & Bilal et al.~\cite{Bilal2018} & \tikzcircle{2pt}                                 & \tikzcircle{2pt}                             & \tikzcircle[black, fill=white]{2pt}                        & \tikzcircle[black, fill=white]{2pt}                             & \tikzcircle{2pt}                        & \tikzcircle[black, fill=white]{2pt}                                   & \tikzcircle{2pt}                         \\ \hline
DeepCompare                & Murugesan et al.~\cite{Murugesan2018} & \tikzcircle{2pt}                                 & \tikzcircle{2pt}                             & \tikzcircle[black, fill=white]{2pt}                        & \tikzcircle[black, fill=white]{2pt}                             & \tikzcircle{2pt}                        & \tikzcircle[black, fill=white]{2pt}                                   & \tikzcircle{2pt}                         \\ \hline
GAN Lab                    & Kahng et al.~\cite{Kahng2018a} & \tikzcircle{2pt}                                 & \tikzcircle[black, fill=white]{2pt}                             & \tikzcircle[black, fill=white]{2pt}                        & \tikzcircle[black, fill=white]{2pt}                             & \tikzcircle{2pt}                        & \tikzcircle[black, fill=white]{2pt}                                   & \tikzcircle{2pt}                         \\ \hline
ActiVis                    & Kahng et al.~\cite{Kahng2018} & \tikzcircle{2pt}                                 & \tikzcircle{2pt}                             & \tikzcircle[black, fill=white]{2pt}                        & \tikzcircle[black, fill=white]{2pt}                             & \tikzcircle{2pt}                        & \tikzcircle[black, fill=white]{2pt}                                   & \tikzcircle{2pt}                         \\ \hline
RetainVis                  & Kwon et al.~\cite{Kwon2018} & \tikzcircle{2pt}                                 & \tikzcircle{2pt}                             & \tikzcircle{2pt}                        & \tikzcircle[black, fill=white]{2pt}                             & \tikzcircle{2pt}                        & \tikzcircle[black, fill=white]{2pt}                                   & \tikzcircle{2pt}                         \\ \hline
LSTMVis                    & Strobelt et al.~\cite{Strobelt2018a} & \tikzcircle{2pt}                                 & \tikzcircle{2pt}                             & \tikzcircle[black, fill=white]{2pt}                        & \tikzcircle[black, fill=white]{2pt}                             & \tikzcircle{2pt}                        & \tikzcircle[black, fill=white]{2pt}                                   & \tikzcircle{2pt}                         \\ \hline
Explanation Explorer       & Krause et al.~\cite{Krause2018} & \tikzcircle{2pt}                                 & \tikzcircle{2pt}                             & \tikzcircle[black, fill=white]{2pt}                        & \tikzcircle{2pt}                             & \tikzcircle{2pt}                        & \tikzcircle[black, fill=white]{2pt}                                   & \tikzcircle{2pt}                         \\ \hline
TF Graph Visualizer        & Wongsuphasawat et al.~\cite{Wongsuphasawat2018} & \tikzcircle{2pt}                                 & \tikzcircle[black, fill=white]{2pt}                             & \tikzcircle[black, fill=white]{2pt}                        & \tikzcircle[black, fill=white]{2pt}                             & \tikzcircle[black, fill=white]{2pt}                        & \tikzcircle[black, fill=white]{2pt}                                   & \tikzcircle{2pt}                         \\ \hline
AEVis                      & Liu et al.\cite{Liu} & \tikzcircle{2pt}                                 & \tikzcircle{2pt}                             & \tikzcircle[black, fill=white]{2pt}                        & \tikzcircle[black, fill=white]{2pt}                             & \tikzcircle{2pt}                        & \tikzcircle[black, fill=white]{2pt}                                   & \tikzcircle{2pt}                         \\ \hline
RuleMatrix                 & Ming et al.~\cite{Ming2019} & \tikzcircle{2pt}                                 & \tikzcircle{2pt}                             & \tikzcircle[black, fill=white]{2pt}                        & \tikzcircle{2pt}                             & \tikzcircle{2pt}                        & \tikzcircle{2pt}                                   & \tikzcircle{2pt}                         \\ \hline
Manifold                   & Zhang et al.~\cite{Zhang2019} & \tikzcircle{2pt}                                 & \tikzcircle{2pt}                             & \tikzcircle[black, fill=white]{2pt}                        & \tikzcircle[black, fill=white]{2pt}                             & \tikzcircle{2pt}                        & \tikzcircle[black, fill=white]{2pt}                                   & \tikzcircle{2pt}                         \\ \hline
DQNViz                     & Wang et al.~\cite{Wang} & \tikzcircle{2pt}                                 & \tikzcircle{2pt}                             & \tikzcircle[black, fill=white]{2pt}                        & \tikzcircle[black, fill=white]{2pt}                             & \tikzcircle{2pt}                        & \tikzcircle[black, fill=white]{2pt}                                   & \tikzcircle{2pt}                         \\ \hline
Seq2Seq-Vis                & Strobelt et al.~\cite{Strobelt2018} & \tikzcircle{2pt}                                 & \tikzcircle{2pt}                             & \tikzcircle[black, fill=white]{2pt}                        & \tikzcircle[black, fill=white]{2pt}                             & \tikzcircle{2pt}                        & \tikzcircle[black, fill=white]{2pt}                                   & \tikzcircle{2pt}                         \\ \hline
IForest                & Zhao et al.~\cite{Zhao2019iforest} & \tikzcircle{2pt}                                 & \tikzcircle{2pt}                             & \tikzcircle[black, fill=white]{2pt}                        & \tikzcircle[black, fill=white]{2pt}                             & \tikzcircle{2pt}                        & \tikzcircle[black, fill=white]{2pt}                                   & \tikzcircle{2pt}                         \\ \hline
IHTM                & El-Assady et al.~\cite{Elassady2018ihtm} & \tikzcircle{2pt}                                 & \tikzcircle{2pt}                             & \tikzcircle{2pt}                        & \tikzcircle[black, fill=white]{2pt}                             & \tikzcircle{2pt}                        & \tikzcircle[black, fill=white]{2pt}                                   & \tikzcircle{2pt}                         \\ \hline
XQuC                      & Sevastjanova et al.~\cite{Sevastjanova2018} & \tikzcircle{2pt}                                 & \tikzcircle{2pt}                             & \tikzcircle{2pt}                        & \tikzcircle{2pt}                             & \tikzcircle{2pt}                        & \tikzcircle[black, fill=white]{2pt}                                   & \tikzcircle{2pt}                         \\ \hline
SMILY                      & Cai et al.~\cite{Cai2019} & \tikzcircle[black, fill=white]{2pt}                                 & \tikzcircle{2pt}                             & \tikzcircle{2pt}                        & \tikzcircle[black, fill=white]{2pt}                             & \tikzcircle{2pt}                        & \tikzcircle{2pt}                                   & \tikzcircle{2pt}                         \\ \hline
\end{tabular}
\caption{VA systems brought into the context of the proposed XAI framework. \textbf{Task} describes the XAI framework tasks. \textbf{Operation Level} shows what the approach needs to complete. In this case, surrogate describes a surrogate model to approximate the decisions of the underlying model. }
\label{tab:vasystems}
\end{table*}

The following section outlines the decisions we took while categorizing the different VA approaches according to \autoref{tab:vasystems} by shortly stating our motives.
Harley~\cite{Harley2015imageinterpreter} show how images can be visualized using the different layers of a network to learn what the networks decides in each step.
Especially, convolutional layers are highlighted to show the transformations they do to an image, solving the task of \emph{understanding}.
Krause et al.~\cite{Krause2016} have a particular focus on feature importance using partial dependency plots~\cite{Friedman2000}. Their visualization show which features are most relevant for a prediction, enabling \emph{understanding} and \emph{diagnosis}.
Liu et al.~\cite{Liu2016} show how it is possible to visualize a convolutional neural network (CNN), supporting users at the identification of possible problems using CNNVis.
They enable the user to \emph{understand}, \emph{diagnose} and later \emph{refine} CNNs for specific tasks.
Rauber et al.~\cite{Rauber16} visualize the training process of a DNN by projecting the layer preceding the output layer to two dimensions. They further display the activation of different neurons to explore the neuron-neuron and neuron-data relationship, focussing on the \emph{understanding} of neurons, but also the \emph{diagnosis} of data and network.
Smilkov et al.~\cite{Smilkov2016tensorflowplayground} use TensorFlow to teach neural network basics to model novices by providing interactive visual analysis.
The TensorFlow Playground has a clear educational focus by letting the user interactively solve problems.
Through this, it supports \emph{understanding}, \emph{diagnosis}, and \emph{refinement}.
Eisemann et al.~\cite{Pezzotti2017} propose a progressive visual analytics system to design deep neural networks, focussing on the underlying layers and on how these change during training.
Thus, DeepEyes has a clear focus on \emph{understanding} and \emph{diagnosis}.
Ming et al.~\cite{Ming2018} provide with RNNVis a novel visualization and analytics system to support the \emph{understanding} of the hidden states of a cell. Furthermore, they \emph{diagnose} dataflow problems of recurrent neural networks.
Liu et al.~\cite{Liu2018} propose DGMTracker to analyze deep generative models, e.g., autoencoders.
It supports experts in \emph{understanding} and \emph{diagnosis} by visualizing different training metrics, dataflow, and activations of layers.
Bilal et al.~\cite{Bilal2018} show the hierarchical abstraction of CNNs visually, enabling \emph{understanding} of the internal representations of CNNs.
Murugesan et al.~\cite{Murugesan2018} enable comparable analytics on two DNNs to understand their corresponding performance, supporting the \emph{diagnosis} of the networks.
Kahng et al.\cite{Kahng2018} propose an industry-scale visual exploration for DNNs to enable users and experts to \emph{understand} and \emph{diagnose} complex deep learning models.
Kahng et al.\cite{Kahng2018a} present GAN Lab, an educational tool focussing on how generative adversarial networks (GAN) work and learn.
They foster an \emph{understanding} of GANs by visualizing the two adversarial networks, highlighting important parts.
Kwon et al.~\cite{Kwon2018} propose RetainVis to allow the interactive exploration of medical data by an improved, interpretable, and interactive RNN-based model called RetainEX. They enable interactive \emph{understanding}, \emph{diagnosis}, and \emph{refinement} of RNNs.
Strobelt et al.~\cite{Strobelt2018a} introduce LSTMVis to explore the inner-workings of LSTM cells. By displaying the hidden cell state and their activations, they support the user to  \emph{understand} and \emph{diagnose} LSTMs.
Krause et al.~\cite{Krause2018} present Model Diagnostics to enable insights into the feature importance of models. They thereby support \emph{understanding} and \emph{diagnosis} of essential features and values.
Wongsuphasawat et al.~\cite{Wongsuphasawat2018} present TF Graph Visualizer. It makes the rendering of large computational graphs possible, helping users to better \emph{understand} the underlying DNN models. 
Liu et al.~\cite{Liu2018} introduce AEVis, a visualization to explore DNNs and their reactions towards adversarial examples.
By highlighting the activation of convolutional layers, they enable \emph{understanding} and \emph{diagnosis} of the sensitivity of CNNs towards adversarial examples.
Ming et al.~\cite{Ming2019} present RuleMatrix, a VA system to explain decisions of a model based on its input-output behavior using rule lists for domain experts with basic ML knowledge.
This method allows to \emph{understand} the model, \emph{diagnose} critical parts, and \emph{report} findings to other researchers with similar problems.
Zhang et al.~\cite{Zhang2019} present Manifold, a model-agnostic framework for interpretation and diagnosis of ML Models, focussing on in- and output of models.
They enable \emph{understanding} and \emph{diagnosis}.
Wang et al.~\cite{Wang} visualize action patterns of reinforcement learning algorithms in games to help model developers to get an intuition for challenges the algorithm could run into, enabling \emph{understanding} and \emph{diagnosis}.
Strobelt et al.~\cite{Strobelt2018} present Seq2Seq-Vis, a tool to interactively explore sequence to sequence models.
By visualizing the attention component of these model structures, they enable \emph{understanding} and \emph{diagnosis}.
Zhao et al.~\cite{Zhao2019iforest} present IForest, a visual system to explore random forest models and predictions by visualizing inherent decision paths, supporting  \emph{understanding} and \emph{diagnosis} for random forests.
El-Assady et al.~\cite{Elassady2018ihtm} introduce an incremental hierarchical topic model, which enables \emph{understanding}, \emph{diagnosis}, and \emph{refinement}. 
Sevastjanova et al.~\cite{Sevastjanova2018} enable model users to improve an explainable classifier through active learning until the classifier reaches a satisfactory level of performance.
XQuC covers \emph{understanding}, \emph{diagnosis}, \emph{refinement}, and \emph{reporting} in a mixed-initiative active learning system. 
Cai et al.~\cite{Cai2019} present SMILY, a medical query application that represents medical images using the embedding of a DNN as a query vector.
\emph{Understanding} of the underlying model is not essential, but to \emph{diagnose} and \emph{refine} the query and the model is.

\begin{landscape}
\section*{Supplementary Study Results}

\begin{table}[!htb]
\centering

\resizebox{1.35\textwidth}{!}{
\begin{tabular}{|p{4cm}|p{4cm}|p{4cm}|p{4cm}|p{4cm}|p{4cm}|p{4cm}|p{4cm}|p{4cm}|p{4cm}|}
\hline
& MN PhD                                          & MN PhD                                                                            & MU PhD                                                                   & MU PhD                                              & MD Student                                            & MD Student                                      & MD Industry                                                             & MD Student                                                     & MD Industry\\
\hline
Prior Knowledge                                 & Never built before but used                                                       & Never built before but used                                              & Never built before but used                         & Never built before but used                           & Built models before                             & Built models before                                                     & Built models before                                            & Built models before                                                                 & Built models before                                                                \\\hline
XAI Use Cases                                   & Analyze Off-the-shelf Models; Gain Trust in Models; Verify Model Functionality;                                                & Understand Model Decisions; Justification of Model Decisions; Gain Trust in Models;  Monitor the Quality of Models;                 & Monitor the Quality of Models; Understand Model Decisions; Improve a Model;   & Analyze Off-the-shelf Models; Gain Trust in Models; Justification of Model Decisions; Monitor the Quality of Models; & Monitor the Quality of Models; Improve a Model;                  & Analyze Off-the-shelf Models; Improve a Model; Justification of Model Decisions; Offer Interpretability of Model;             & Justification of Model Decisions; Detect Model Biases; Show Feature Influence on Decision; Show Model Decision to Clients;                & Marketing for Models; Monitor the Quality of Models; Iteratively Build Models; Improve a Model;                                 & Understand Model Decisions; Monitor the Quality of Models;                                               \\\hline
Review of Framework                             & Pipeline Makes Sense for Engineering Tasks; Add a Model Building Phase; Merge Understanding and Diagnosis;                                           & Pipeline Makes Sense for Engineering Tasks; Merge Understanding and Diagnosis;                                                &                                                     & Pipeline Makes Sense for Engineering Tasks;                                     &                                                 &                                                                         & Input Domain Feedback during Refinement; Conduct the Refinement Independent of XAI; Merge Understanding and Diagnosis;                    & Pipeline Makes Sense for Engineering Tasks; Merge Understanding and Diagnosis;                                                           & Pipeline Makes Sense for Engineering Tasks;                                                                  \\\hline
Understanding           & Sync Graph State Globally; Show Image before Wiki-Explainer; Show a Simple Graph Layout; See TB Graph after Simple Graph; Show Dataflow Graph; Show Textual Graph Summary; & Show a Simple Graph Layout; Show Dataflow Graph;                                                    & Show a Simple Graph Layout; See TB Graph after Simple Graph;                         & Show Numeric Parameters in Graph; Show a Simple Graph Layout; Compare Pretrained Model Architectures;  & Show Image before Wiki-Explainer; Show Numeric Parameters in Graph; Verify Architecture of Model; & Sync Graph State Globally; Show Numeric Parameters in Graph; Show the Model Code; Show a Simple Graph Layout; Show Dataflow Graph; Show Textual Graph Summary; & Show Numeric Parameters in Graph; Show Textual Graph Summary; Show a Simple Graph Layout; See TB Graph after Simple Graph; & Show Dataflow Graph;                                                                            & Wiki-Explainer is Useful; For Own Code No Understanding Needed; Compare Pretrained Model Architectures;                                      \\\hline
Diagnosis  & Relate Explainer Output to Domain Knowledge; Understand Model Decisions; Offer Data Inspection as Explainer;                        & Diagnosing with Many Explainers is Useful; See Convergence of Training as Explainer;                                                      & See Convergence of Training as Explainer; Suggest Recently Used Explainers for new Model;            &                                                       & Diagnosing with Many Explainers is Useful; Diagnosis is the Most Important Task;                          & Diagnosing with Many Explainers is Useful; Diagnosis is the Most Important Task; Offer Data Inspection as Explainer;                           & Diagnosis is the Most Important Task;                                              &                                                                                     & Scalability of Explainers to Big Models; TB Needs Predefined Scopes;                                                       \\\hline
XAI & Gain Insights into how Explainers Work; Explainers are too Complex; Explain a Sample/Class At Once; Explain Multiple Samples at Once; Do not Trust Explainer Results;               & Do not Trust Explainer Results; Reference the Origin of Explainers; Suggest Explainers fitting the Data/Model/History;                      & HistoTrend Explainer is Helpful; Low-Abstraction Explainers are Helpful;                            & Explain Multiple Samples at Once; Use Global Explainers on Intermediate Layers;      & Explainer for Comparison of Explainers; Reference the Origin of Explainers;               & Gain Insights into how Explainers Work; Do not Trust Explainer Results; Explain Multiple Samples at Once; Explain a Sample/Class At Once;                & Gain Insights into how Explainers Work; Do not Trust Explainer Results;                                     & Gain Insights into how Explainers Work; Add more Explainers; Do not Trust Explainer Results;                                          & Explain Multiple Samples at Once; Reference the Origin of Explainers; Use Global Explainers on Intermediate Layers; Do not Trust Explainer Results; \\\hline
Metrics    & Use Metrics as Explainer on Parts of the Model; Use Metrics as Explainer in Diagnosis;                                                      &                                                                          &                                                     & Show Metrics in Report on Model; Use Metrics as Explainer in Diagnosis;                         & Show Metrics during Refinement; Use Metrics as Explainer in Diagnosis;               & Show Metrics during Refinement; Use Metrics as Explainer in Diagnosis;                                       & Use Metrics as Explainer in Diagnosis;                                                & Use Metrics as Explainer in Diagnosis;                                                                     & Use the Explainer as an Additional Quality Metric;                                                          \\\hline
Refinement       & Show/Modify Model with Building Blocks; Add More Data; Change Input Features;                                             & Add More Data; Change Hyper Parameters; Retrain and Remove Layers;                        &                                                     & Add More Data; Change Hyper Parameters; Suggest Refinements based on Rules;                & Suggest Refinements based on Rules; Click-To-Refine is Impressive but Doubtful;        & Add More Data; Propose Code Snippets To Add to Model; Change Hyper Parameters;                       &                                                                & Click-To-Refine is Impressive but Doubtful; Click-To-Refine is Unrealistic; Copyright Issues with Code suggested in Refinement; Editor Needed to Describe the Refinements; Propose Code Snippets To Add to Model; Add More Data; & Refinements should link to TB Example Code;                                                                   \\\hline
Model Comparison & Highlight Difference between Graphs; Compare Multipe Model Configurations at Once; Compare Models with Speculative Execution; Show/Modify Model with Building Blocks;                       &                                                                          & Sync Graph State Globally; Highlight Difference between Graphs; Show Models in Parallel for Comparison; &                                                       & Compare Multipe Model Configurations at Once; Compare Models with Speculative Execution;                               & Compare Multipe Model Configurations at Once; Compare Models with Speculative Execution; Show/Modify Model with Building Blocks;                                        & Compare Multipe Model Configurations at Once; Compare Models with Speculative Execution; Show/Modify Model with Building Blocks;                               & Compare Multipe Model Configurations at Once;                                                                          & Show Models in Parallel for Comparison;                                                                     \\\hline
Provenance Tracking            & Sync Graph State Globally; Annotate Provenance Cards; Group Provenance Cards;                                               & Add Graph Snapshot to Provenance; Annotate Provenance Cards; Compare Explainer Output in Provenance; Group Provenance Cards; Add Wiki-Explainers to Provenance; & Annotate Provenance Cards; Compare Explainer Output in Provenance; Group Provenance Cards;             & Add Graph Snapshot to Provenance; Annotate Provenance Cards; Compare Explainer Output in Provenance; Group Provenance Cards;  & Bookmark Current Explainer Selection; Group Provenance Cards;                            & Compare Explainer Output in Provenance;                                                           & Annotate Provenance Cards; Compare Explainer Output in Provenance; Group Provenance Cards;                        &                                                                                     & Compare Explainer Output in Provenance; Group Provenance Cards; RerunExplainers in Provenance with New Model; Annotate Provenance Cards; Enlarge Provenance Card; Reload Explainer from Provenance Cards;           \\\hline
Reporting    & Share with Colleagues; Justification of Model Decisions; Store Analysis Report instead of Memorizing; Annotate Within Report;                                           & Justification of Model Decisions; Show an Overview of the Model Comparison; Share with Stakeholders; Store Analysis Report instead of Memorizing;                & Export Report as PDF;                                                 & Share with Colleagues; Store Analysis Report instead of Memorizing; Justification of Model Decisions; Annotate Within Report;              & Show an Overview of the Model Comparison; Share with Colleagues; Export Report as PDF; Send Report via Mail;      & Share with Colleagues; Show an Overview of the Model Comparison;                                      & Show an Overview of the Model Comparison; Share with Colleagues; Share Report on ML Pattern Forums;                & Export Report as SVG; Share with Colleagues; Share Report on ML Pattern Forums; Show an Overview of the Model Comparison;                                 & Export Report to Paper; Export Report as SVG; Export Report as PDF;                                                          \\\hline
Overall Impression                              & System is rich in Features; System is Helpful;                                                               & System is Valuable;                                                                 & System is Valuable;                                            & System is Valuable;                                              & System is Valuable;                                        & System Offers Nice Interactivity;                                                         & System is Valuable;                                                       & System Offers Nice Interactivity;                                                                     & System is Valuable;\\\hline
Other Users                                     & Too Complex for Beginners;                                                                &                                                                          & System Could be used by Model Users; Too Complex for Beginners;                      & System Could be used by Model Users; System Could be Playground for Students;                        & Only Usable for Developers;                                         & Too Complex for Beginners;                                                      & Too Complex for Beginners;                                             & System Could be Playground for Students;                                                                   &                                                                                    \\\hline
User Guidance                                   & Show Starting Point In Tool; Show Examples of Stereotypical Architectures;                                                    & Tutorial before first System Usage;                                                                 & Show Starting Point In Tool; Tutorial before first System Usage; Show a Task Checklist;                       & More Infolabels in UI;                                             &                                                 & Show Starting Point In Tool; Tutorial before first System Usage; Show a Task Checklist;                                           &                                                                &                                                                                  & More Infolabels in UI;                                                                          \\\hline
\end{tabular}
}
\caption{Overview of topics collected from each participant in the qualitative evaluation.}
\label{tab:study}
\end{table}

\end{landscape}

\begin{figure*}[b]
    \centering
    \captionsetup{justification=centering}
    \includegraphics[width=0.475\textwidth]{figures/study/0StudyDataSquare_5_part1.png}
    \quad
    \includegraphics[width=0.475\textwidth]{figures/study/0StudyDataSquare_5_part2.png}
    \caption{Summary of response counts for each user type during the study.\\ Model novices in orange, model users in blue, and model developers in green.}
    \label{fig:studydatasquare}
\end{figure*}
