# Supplementary material for: explAIner: A Visual Analytics Framework for Interactive and Explainable Machine Learning
Source: arXiv:1908.00087 ancillary file (2019-10-07)
Supplement: Supplementary file 2 [file explainer_supplementary-material.pdf]

# explAIner: A Visual Analytics Framework for Interactive and Explainable Machine Learning

## Supplementary Material

Thilo Spinner, Udo Schlegel, Hanna Schäfer, and Mennatallah El-Assady

---

### SUPPLEMENTARY RELATED WORK

The following section outlines the decisions we took while categorizing the different VA approaches according to Table S1 by shortly stating our motives.

Harley [5] show how images can be visualized using the different layers of a network to learn what the networks decides in each step. Especially, convolutional layers are highlighted to show the transformations they do to an image, solving the task of *understanding*.

Krause et al. [9] have a particular focus on feature importance using partial dependency plots [4]. Their visualization show which features are most relevant for a prediction, enabling *understanding* and *diagnosis*.

Liu et al. [13] show how it is possible to visualize a convolutional neural network (CNN), supporting users at the identification of possible problems using CNNVis. They enable the user to *understand*, *diagnose* and later *refine* CNNs for specific tasks.

Rauber et al. [18] visualize the training process of a DNN by projecting the layer preceding the output layer to two dimensions. They further display the activation of different neurons to explore the neuron-neuron and neuron-data relationship, focussing on the *understanding* of neurons, but also the *diagnosis* of data and network.

Smilkov et al. [20] use TensorFlow to teach neural network basics to model novices by providing interactive visual analysis. The TensorFlow Playground has a clear educational focus by letting the user interactively solve problems. Through this, it supports *understanding*, *diagnosis*, and *refinement*.

Eisemann et al. [17] propose a progressive visual analytics system to design deep neural networks, focussing on the underlying layers and on how these change during training. Thus, DeepEyes has a clear focus on *understanding* and *diagnosis*.

Ming et al. [14] provide with RNNVis a novel visualization and analytics system to support the *understanding* of the hidden states of a cell. Furthermore, they *diagnose* dataflow problems of recurrent neural networks.

Liu et al. [12] propose DGMTracker to analyze deep generative models, e.g., autoencoders. It supports experts in *understanding* and *diagnosis* by visualizing different training metrics, dataflow, and activations of layers.

Bilal et al. [1] show the hierarchical abstraction of CNNs visually, enabling *understanding* of the internal representations of CNNs.

Murugesan et al. [16] enable comparable analytics on two DNNs to understand their corresponding performance, supporting the *diagnosis* of the networks.

Kahng et al. [6] propose an industry-scale visual exploration for DNNs to enable users and experts to *understand* and *diagnose* complex deep learning models.

Kahng et al. [7] present GAN Lab, an educational tool focussing on how generative adversarial networks (GAN) work and learn. They

foster an *understanding* of GANs by visualizing the two adversarial networks, highlighting important parts.

Kwon et al. [10] propose RetainVis to allow the interactive exploration of medical data by an improved, interpretable, and interactive RNN-based model called RetainEX. They enable interactive *understanding*, *diagnosis*, and *refinement* of RNNs.

Strobelt et al. [22] introduce LSTMVis to explore the inner-workings of LSTM cells. By displaying the hidden cell state and their activations, they support the user to *understand* and *diagnose* LSTMs.

Krause et al. [8] present Model Diagnostics to enable insights into the feature importance of models. They thereby support *understanding* and *diagnosis* of essential features and values.

Wongsuphasawat et al. [24] present TF Graph Visualizer. It makes the rendering of large computational graphs possible, helping users to better *understand* the underlying DNN models.

Liu et al. [12] introduce AEVis, a visualization to explore DNNs and their reactions towards adversarial examples. By highlighting the activation of convolutional layers, they enable *understanding* and *diagnosis* of the sensitivity of CNNs towards adversarial examples.

Ming et al. [15] present RuleMatrix, a VA system to explain decisions of a model based on its input-output behavior using rule lists for domain experts with basic ML knowledge. This method allows to *understand* the model, *diagnose* critical parts, and *report* findings to other researchers with similar problems.

Zhang et al. [25] present Manifold, a model-agnostic framework for interpretation and diagnosis of ML Models, focussing on in- and output of models. They enable *understanding* and *diagnosis*.

Wang et al. [23] visualize action patterns of reinforcement learning algorithms in games to help model developers to get an intuition for challenges the algorithm could run into, enabling *understanding* and *diagnosis*.

Strobelt et al. [21] present Seq2Seq-Vis, a tool to interactively explore sequence to sequence models. By visualizing the attention component of these model structures, they enable *understanding* and *diagnosis*.

Zhao et al. [26] present IForest, a visual system to explore random forest models and predictions by visualizing inherent decision paths, supporting *understanding* and *diagnosis* for random forests.

El-Assady et al. [3] introduce an incremental hierarchical topic model, which enables *understanding*, *diagnosis*, and *refinement*.

Sevastjanova et al. [19] enable model users to improve an explainable classifier through active learning until the classifier reaches a satisfactory level of performance. XQuC covers *understanding*, *diagnosis*, *refinement*, and *reporting* in a mixed-initiative active learning system.

Cai et al. [2] present SMILY, a medical query application that represents medical images using the embedding of a DNN as a query vector. *Understanding* of the underlying model is not essential, but to *diagnose* and *refine* the query and the model is.

| VA Approach           | Reference                  | Task     |           |            |           | Operation Level |           |       |
|-----------------------|----------------------------|----------|-----------|------------|-----------|-----------------|-----------|-------|
|                       |                            | Underst. | Diagnosis | Refinement | Reporting | Data            | Surrogate | Model |
| Node-Link Vis         | Harley [5]                 | ●        | ○         | ○          | ○         | ●/○             | ○         | ●     |
| Prospector            | Krause et al. [9]          | ●        | ●         | ○          | ○         | ●               | ○         | ●     |
| CNNVis                | Liu et al. [13]            | ●        | ●         | ●          | ○         | ●               | ○         | ●     |
| Hidden Activity Vis   | Rauber et al. [18]         | ●        | ●         | ○          | ○         | ●               | ○         | ●     |
| TensorFlow Playground | Smilkov et al. [20]        | ●        | ●         | ●          | ○         | ●               | ○         | ●     |
| DeepEyes              | Pezzoti et al. [17]        | ●        | ●         | ●          | ○         | ●               | ○         | ●     |
| RNNVis                | Ming et al. [14]           | ●        | ●         | ○          | ○         | ●               | ○         | ●     |
| DGMTracker            | Liu et al. [12]            | ●        | ●         | ○          | ○         | ●               | ○         | ●     |
| Class Hierarchy?      | Bilal et al. [1]           | ●        | ●         | ○          | ○         | ●               | ○         | ●     |
| DeepCompare           | Murugesan et al. [16]      | ●        | ●         | ○          | ○         | ●               | ○         | ●     |
| GAN Lab               | Kahng et al. [7]           | ●        | ○         | ○          | ○         | ●               | ○         | ●     |
| ActiVis               | Kahng et al. [6]           | ●        | ●         | ○          | ○         | ●               | ○         | ●     |
| RetainVis             | Kwon et al. [10]           | ●        | ●         | ●          | ○         | ●               | ○         | ●     |
| LSTMVis               | Strobelt et al. [22]       | ●        | ●         | ○          | ○         | ●               | ○         | ●     |
| Explanation Explorer  | Krause et al. [8]          | ●        | ●         | ○          | ●         | ●               | ○         | ●     |
| TF Graph Visualizer   | Wongsuphasawat et al. [24] | ●        | ○         | ○          | ○         | ○               | ○         | ●     |
| AEVis                 | Liu et al. [11]            | ●        | ●         | ○          | ○         | ●               | ○         | ●     |
| RuleMatrix            | Ming et al. [15]           | ●        | ●         | ○          | ●         | ●               | ●         | ●     |
| Manifold              | Zhang et al. [25]          | ●        | ●         | ○          | ○         | ●               | ○         | ●     |
| DQNViz                | Wang et al. [23]           | ●        | ●         | ○          | ○         | ●               | ○         | ●     |
| Seq2Seq-Vis           | Strobelt et al. [21]       | ●        | ●         | ○          | ○         | ●               | ○         | ●     |
| IForest               | Zhao et al. [26]           | ●        | ●         | ○          | ○         | ●               | ○         | ●     |
| IHTM                  | El-Assady et al. [3]       | ●        | ●         | ●          | ○         | ●               | ○         | ●     |
| XQuC                  | Sevastjanova et al. [19]   | ●        | ●         | ●          | ●         | ●               | ○         | ●     |
| SMILY                 | Cai et al. [2]             | ○        | ●         | ●          | ○         | ●               | ●         | ●     |

Table S1: VA systems brought into the context of the proposed XAI framework. **Task** describes the XAI framework tasks. **Operation Level** shows what the approach needs to complete. In this case, surrogate describes a surrogate model to approximate the decisions of the underlying model.

## SUPPLEMENTARY STUDY RESULTS

|                                   |                                                                                                                                                                                        |                                                                                                                                                                |                                                                                                                               |                                                                                                                                                       |                                                                                                                                                        |                                                                                                                                                                                                  |                                                                                                                                                                                                             |                                                                                                  |
|-----------------------------------|----------------------------------------------------------------------------------------------------------------------------------------------------------------------------------------|----------------------------------------------------------------------------------------------------------------------------------------------------------------|-------------------------------------------------------------------------------------------------------------------------------|-------------------------------------------------------------------------------------------------------------------------------------------------------|--------------------------------------------------------------------------------------------------------------------------------------------------------|--------------------------------------------------------------------------------------------------------------------------------------------------------------------------------------------------|-------------------------------------------------------------------------------------------------------------------------------------------------------------------------------------------------------------|--------------------------------------------------------------------------------------------------|
| Prior Knowledge<br>XXAI Use Cases | Never built before but used<br>Analyze Off-the-shelf Models;<br>Gain Trust in Models; Verify Model Functionality;                                                                      | MN PHD<br>Never built before but used<br>Understand Model Decisions;<br>Justification of Model Decisions; Gain Trust in Models; Monitor the Quality of Models; | MU PHD<br>Monitor the Quality of Models; Understand Model Decisions; Improve a Model;                                         | MD Student<br>Monitor the Quality of Models; Improve a Model; Justification of Model Decisions; Offer Interpretability of Model;                      | MD Student<br>Build models before<br>Analyze Off-the-shelf Models; Improve a Model; Justification of Model Decisions; Offer Interpretability of Model; | MD Industry<br>Build models before<br>Justification of Model Decisions; Detect Model Biases; Show Feature Influence on Decision; Show Model Decision to Clients;                                 | MD Student<br>Build models before<br>Marketing for Models; Monitor the Quality of Models; Iteratively Build Models; Improve a Model;                                                                        | MD Industry<br>Build models before<br>Understand Model Decisions; Monitor the Quality of Models; |
|                                   | Pipeline Makes Sense for Engineering Tasks; Add a Model Building Phase; Merge Understanding and Diagnosis;                                                                             | Pipeline Makes Sense for Engineering Tasks;                                                                                                                    | Pipeline Makes Sense for Engineering Tasks;                                                                                   | Pipeline Makes Sense for Engineering Tasks; Monitor the Quality of Models;                                                                            | Input Domain Feedback during Refinement; Conduct the Refinement Independent of XXAI; Merge Understanding and Diagnosis;                                | Pipeline Makes Sense for Engineering Tasks; Merge Understanding and Diagnosis;                                                                                                                   | Pipeline Makes Sense for Engineering Tasks;                                                                                                                                                                 |                                                                                                  |
| Understanding                     | Sync Graph State Globally; Show Image before Wiki-Explainer; Show a Simple Graph Layout; See TB Graph after Simple Graph; Show Datalow Graph; Show Textual Graph Summary;              | Show a Simple Graph Layout; See TB Graph after Simple Graph;                                                                                                   | Show Numeric Parameters in Graph; Compare Pretrained Model Architectures;                                                     | Sync Graph State Globally; Show Numeric Parameters in Graph; Show Textual Graph Summary; Show a Simple Graph Layout; See TB Graph after Simple Graph; | Sync Numeric Parameters in Graph; Show Textual Graph Summary; Show a Simple Graph Layout; See TB Graph after Simple Graph;                             | Show Datalow Graph;                                                                                                                                                                              | Wiki-Explainer is Useful; For Own Code No Understanding Needed; Compare Pretrained Model Architectures;                                                                                                     |                                                                                                  |
| Diagnosis                         | Diagnosing with Many Explainers is Useful; See Convergence of Training as Explainer; Suggest Recently Used Explainers for new Model;                                                   | See Convergence of Training as Explainer; Suggest Recently Used Explainers for new Model;                                                                      |                                                                                                                               | Diagnosing with Many Explainers is Useful; Diagnosis is the Most Important Task; Offer Data Inspection as Explainer;                                  | Diagnosis is the Most Important Task;                                                                                                                  |                                                                                                                                                                                                  | Scalability of Explainers to Big Models; TB Needs Predefined Scopes;                                                                                                                                        |                                                                                                  |
| XXAI                              | Gain Insights into how Explainers Work; Explainers are too Complex; Explain a Simple Class At Once; Do not Trust Explainer Results; Suggest Explainers fitting the Data/Model/History; | Do not Trust Explainer Results; Reference the Origin of Explainers; Suggest Explainers fitting the Data/Model/History;                                         | Explain Multiple Samples at Once; Use Global Explainers on Intermediate Layers;                                               | Gain Insights into how Explainers Work; Do not Trust Explainer Results; Explain Multiple Samples at Once; Explain a Sample/Class At Once;             | Gain Insights into how Explainers Work; Do not Trust Explainer Results;                                                                                | Gain Insights into how Explainers Work; Add more Explainers; Do not Trust Explainer Results;                                                                                                     | Explain Multiple Samples at Once; Reference the Origin of Explainers; Use Global Explainers on Intermediate Layers; Do not Trust Explainer Results;                                                         |                                                                                                  |
| Metrics                           | Use Metrics as Explainer on Parts of the Model; Use Metrics as Explainer in Diagnosis;                                                                                                 | Show Metrics in Report on Model; Use Metrics as Explainer in Diagnosis;                                                                                        |                                                                                                                               | Show Metrics during Refinement; Use Metrics as Explainer in Diagnosis;                                                                                | Use Metrics as Explainer in Diagnosis;                                                                                                                 | Use Metrics as Explainer in Diagnosis;                                                                                                                                                           | Use the Explainer as an Additional Quality Metric;                                                                                                                                                          |                                                                                                  |
| Refinement                        | Show/Modify Model with Building Blocks; Add More Data; Change Input Features;                                                                                                          | Add More Data; Change Hyper Parameters; Retrain and Remove Layers;                                                                                             |                                                                                                                               | Add More Data; Propose Code Snippets To Add to Model; Change Hyper Parameters;                                                                        |                                                                                                                                                        | Click-To-Rename is Impressive but Doubtful; Copyright Issues with Code suggested in Refinement; Editor Needed to Describe the Refinements; Propose Code Snippets To Add to Model; Add More Data; | Refinements should link to TB Example Code;                                                                                                                                                                 |                                                                                                  |
| Model Comparison                  | Highlight Difference between Graphs; Compare Multiple Model Configurations at Once; Compute Models with Speculative Execution; Show/Modify Model with Building Blocks;                 | Sync Graph State Globally; Highlight Difference between Graphs; Show Models in Parallel for Comparison;                                                        |                                                                                                                               | Compare Multiple Model Configurations at Once; Compare Models with Speculative Execution; Show/Modify Model with Building Blocks;                     | Compare Multiple Model Configurations at Once; Compare Models with Speculative Execution; Show/Modify Model with Building Blocks;                      | Compare Multiple Model Configurations at Once;                                                                                                                                                   | Show Models in Parallel for Comparison;                                                                                                                                                                     |                                                                                                  |
| Provenance Tracking               | Sync Graph State Globally; Annotate Provenance Cards; Group Provenance Cards;                                                                                                          | Add Graph Snapshot to Provenance; Annotate Provenance Cards; Compare Explainer Output in Provenance; Group Explainers to Provenance;                           | Add Graph Snapshot to Provenance; Annotate Provenance Cards; Compare Explainer Output in Provenance; Group Provenance Cards;  | Compare Explainer Output in Provenance;                                                                                                               | Annotate Provenance Cards; Compare Explainer Output in Provenance; Group Provenance Cards;                                                             |                                                                                                                                                                                                  | Compare Explainer Output in Provenance; Group Provenance Cards; Rename Explainers in Provenance with New Model; Annotate Provenance Cards; Enlarge Provenance Card; Reload Explainer from Provenance Cards; |                                                                                                  |
| Reporting                         | Share with Colleagues; Justification of Model Decisions; Store Analysis Report instead of Memorizing; Justification of Model Decisions; Annotate Within Report;                        | Export Report as PDF;                                                                                                                                          | Share with Colleagues; Store Analysis Report instead of Memorizing; Justification of Model Decisions; Annotate Within Report; | Share with Colleagues; Show an Overview of the Model Comparison;                                                                                      | Share with Colleagues; Show an Overview of the Model Comparison; Share with Colleagues; Export Report as PDF; Send Report via Mail;                    | Export Report as SVG; Share Report with Colleagues; Show on ML Pattern Forums; Show an Overview of the Model Comparison;                                                                         | Export Report to Paper; Export Report as SVG; Export Report as PDF;                                                                                                                                         |                                                                                                  |
| Overall Impression                | System is rich in Features; System is Helpful;                                                                                                                                         | System is Valuable;                                                                                                                                            | System is Valuable;                                                                                                           | System Offers Nice Interactivity; Too Complex for Beginners;                                                                                          | System Offers Nice Interactivity; Too Complex for Beginners;                                                                                           | System Offers Nice Interactivity; Too Complex for Beginners;                                                                                                                                     | System is Valuable;                                                                                                                                                                                         |                                                                                                  |
| Other Users                       | Too Complex for Beginners;                                                                                                                                                             | System Could be used by Model Users; Too Complex for Beginners;                                                                                                | System Could be used by Model Users; System Could be Playground for Students;                                                 | Too Complex for Beginners;                                                                                                                            | Too Complex for Beginners;                                                                                                                             | System Could be Playground for Students;                                                                                                                                                         |                                                                                                                                                                                                             |                                                                                                  |
| User Guidance                     | Show Starting Point In Tool; Show Examples of Stereotypical Architectures;                                                                                                             | Tutorial before first System Usage;                                                                                                                            | Show Starting Point In Tool; Tutorial before first System Usage; Show a Task Checklist;                                       | Show Starting Point In Tool; Tutorial before first System Usage; Show a Task Checklist;                                                               |                                                                                                                                                        |                                                                                                                                                                                                  | More Infotabls in UI;                                                                                                                                                                                       |                                                                                                  |

Table S2: Overview of topics collected from each participant in the qualitative evaluation.

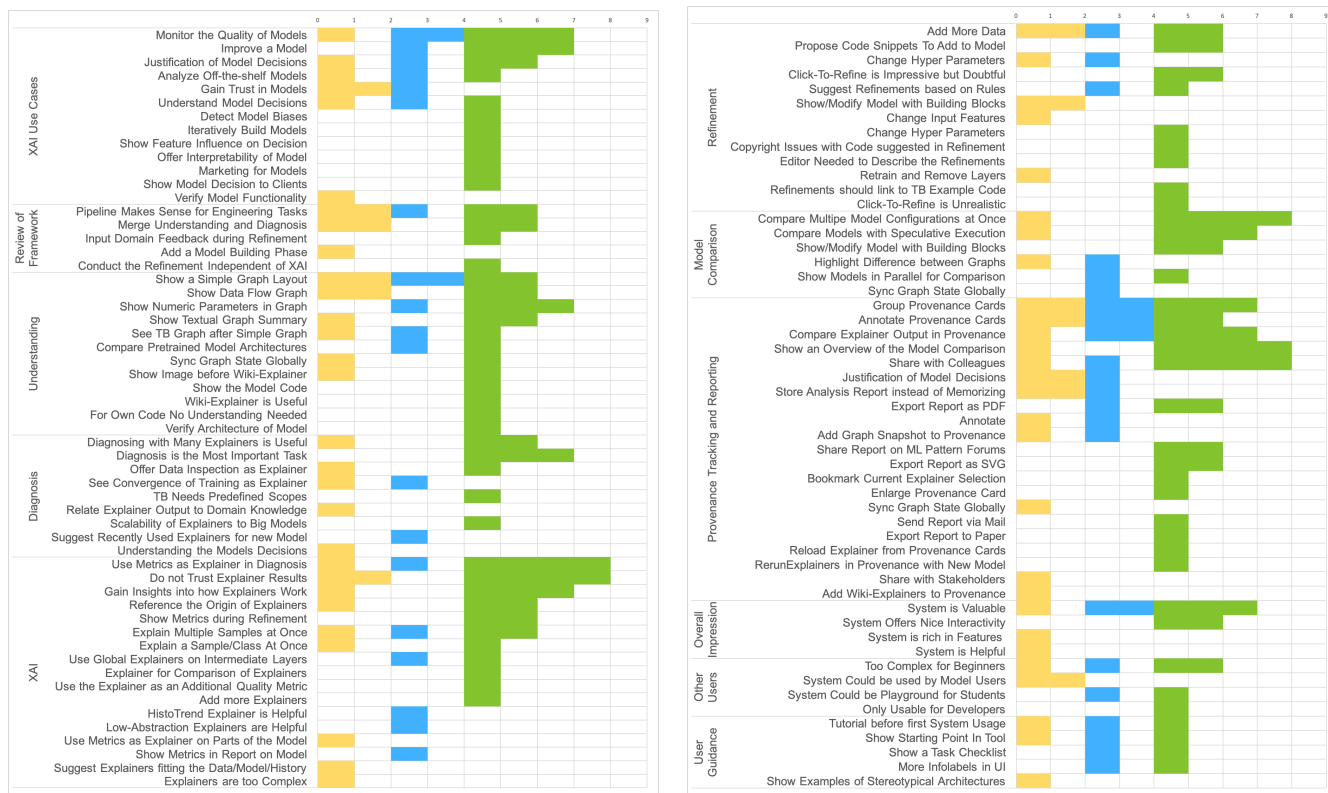

Fig. S1: Summary of response counts for each user type during the study. Model novices in orange, model users in blue, and model developers in green.

## REFERENCES

- [1] A. Bilal, A. Jourabloo, M. Ye, X. Liu, and L. Ren. Do Convolutional Neural Networks Learn Class Hierarchy? *IEEE Trans. Vis. Comput. Graph.*, 2018.
- [2] C. Cai, E. Reif, N. Hegde, J. Hipp, B. Kim, D. Smilkov, M. Wattenberg, D. Viegas, G. Corrado, M. Stumpe, and M. Terry. Human-Centered Tools for Coping with Imperfect Algorithms during Medical Decision-Making. *CHI Conf. Hum. Factors Comput. Syst.*, 2019.
- [3] M. El-Assady, F. Sperrle, O. Deussen, D. Keim, and C. Collins. Visual Analytics for Topic Model Optimization based on User-Steerable Speculative Execution. *IEEE Trans. Vis. Comput. Graph.*, 2019.
- [4] J. Friedman. Greedy Function Approximation: A Gradient Boosting Machine. *Ann. Stat.*, 2000.
- [5] A. Harley. An Interactive Node-Link Visualization of Convolutional Neural Networks. In *ISVC*, 2015.
- [6] M. Kahng, P. Andrews, A. Kalro, and D. Chau. ActiVis: Visual Exploration of Industry-Scale Deep Neural Network Models. *IEEE Trans. Vis. Comput. Graph.*, 2018.
- [7] M. Kahng, N. Thorat, D. Chau, F. Viegas, and M. Wattenberg. GAN Lab: Understanding Complex Deep Generative Models using Interactive Visual Experimentation. *IEEE Trans. Vis. Comput. Graph.*, 2018.
- [8] J. Krause, A. Dasgupta, J. Swartz, Y. Aphinyanaphongs, and E. Bertini. A Workflow for Visual Diagnostics of Binary Classifiers using Instance-Level Explanations. *IEEE Conf. Vis. Anal. Sci. Technol.*, 2018.
- [9] J. Krause, A. Perer, and K. Ng. Interacting with Predictions: Visual Inspection of Black-box Machine Learning Models. In *CHI Conf. Hum. Factors Comput. Syst.*, 2016.
- [10] B. Kwon, M. Choi, J. Kim, E. Choi, Y. Kim, S. Kwon, J. Sun, and J. Choo. RetainVis: Visual Analytics with Interpretable and Interactive Recurrent Neural Networks on Electronic Medical Records. *IEEE Trans. Vis. Comput. Graph.*, 2018.
- [11] M. Liu, S. Liu, H. Su, K. Cao, and J. Zhu. Analyzing the Noise Robustness of Deep Neural Networks. *arXiv Prepr. arXiv1810.03913*, 2018.
- [12] M. Liu, J. Shi, K. Cao, J. Zhu, and S. Liu. Analyzing the Training Processes of Deep Generative Models. *IEEE Trans. Vis. Comput. Graph.*, 2018.
- [13] M. Liu, J. Shi, Z. Li, C. Li, J. Zhu, and S. Liu. Towards Better Analysis of Deep Convolutional Neural Networks. *IEEE Trans. Vis. Comput. Graph.*, 2017.
- [14] Y. Ming, S. Cao, R. Zhang, Z. Li, Y. Chen, Y. Song, and H. Qu. Understanding Hidden Memories of Recurrent Neural Networks. *EEE Conf. Vis. Anal. Sci. Technol.*, 2018.
- [15] Y. Ming, H. Qu, and E. Bertini. RuleMatrix: Visualizing and Understanding Classifiers with Rules. *IEEE Trans. Vis. Comput. Graph.*, 2019.
- [16] S. Murugesan, S. Malik, F. Du, E. Koh, and T. Lai. DeepCompare : Visual and Interactive Comparison of Deep Learning Model Performance. In *Symp. Vis. Data Sci.*, 2018.
- [17] Pezzotti, N. and Holtt, T. and Van Gemert, J. and Lelieveldt, B.P.F. and Eisemann, E. and Vilanova, A. DeepEyes: Progressive Visual Analytics for Designing Deep Neural Networks. *IEEE Trans. Vis. Comput. Graph.*, 2017.
- [18] P. Rauber, S. Fadel, and Falcão, A.X. and Telea, A.C. Visualizing the Hidden Activity of Artificial Neural Networks. *IEEE Trans. Vis. Comput. Graph.*, 2017.
- [19] R. Sevastjanova, M. El-Assady, A. Hautli-Janisz, A. Kalouli, R. Kehlbeck, O. Deussen, D. Keim, and M. Butt. Mixed-initiative active learning for generating linguistic insights in question classification. *IEEE VIS Work. Data Syst. Interact. Anal.*, 2018.
- [20] D. Smilkov, S. Carter, D. Sculley, and Viégas, F.B. and Wattenberg, M. Direct-Manipulation Visualization of Deep Networks. In *ICML Work. Vis. Deep Learn.*, 2016.
- [21] H. Strobelt, S. Gehrmann, M. Behrisch, A. Perer, H. Pfister, and A. Rush. Seq2seq-Vis: A Visual Debugging Tool for Sequence-to-Sequence Models. *IEEE Trans. Vis. Comput. Graph.*, 2019.
- [22] H. Strobelt, S. Gehrmann, H. Pfister, and A. Rush. LSTMVis: A Tool for Visual Analysis of Hidden State Dynamics in Recurrent Neural Networks. *IEEE Trans. Vis. Comput. Graph.*, 2018.
- [23] J. Wang, L. Gou, H. Shen, and H. Yang. DQNViz: A Visual Analytics Approach to Understand Deep Q-Networks. *IEEE Trans. Vis. Comput. Graph.*, 2019.
- [24] K. Wongsuphasawat, D. Smilkov, J. Wexler, J. Wilson, and Mané, D. and Fritz, D. and Krishnan, D. and Viégas, F.B. and Wattenberg, M. Visualizing Dataflow Graphs of Deep Learning Models in TensorFlow. *IEEE Trans. Vis. Comput. Graph.*, 2018.
- [25] J. Zhang, Y. Wang, P. Molino, L. Li, and D. Ebert. Manifold: A Model-Agnostic Framework for Interpretation and Diagnosis of Machine Learning Models. *IEEE Trans. Vis. Comput. Graph.*, 2019.
- [26] X. Zhao, Y. Wu, D. Lee, and W. Cui. IForest: Interpreting Random Forests via Visual Analytics. *IEEE Trans. Vis. Comput. Graph.*, 2019.
